# Supplementary material for: An Efficient and Balanced Graph Partition Algorithm for the Subgraph-Centric Programming Model on Large-scale Power-law Graphs
Source: arXiv:2010.09007 source file (2021-07-07)
Supplement: Supplementary file 1 [file appendix.tex]

\appendices
\section{}\label{app:alpha}
\begin{theorem}
	Partitioning graph $G(V, E)$ into $p$ partitions by our EBG algorithm, the upper bound of the edge imbalance factor is $1 + \frac{p-1}{|E|} (1 + \lfloor \frac{2|E|}{\alpha p} + \frac{\beta}{\alpha} |E| \rfloor$.
\end{theorem}

\begin{proof}
	For the sake of simplicity, we denote $Score^m_{(u, v)}(i)$, $e_{count}^m[i]$, $v_{count}^m[i]$ and $keep^m[i]$ as the value of $Score_{(u, v)}(i)$, $e_{count}[i]$, $v_{count}[i]$ and $keep[i]$ before assigning the $m^{th}$ edge, while $m \in [1, |E|]$.
	Specifically, $e_{count}^{|E| + 1}[i]$ are denoted as $|E_i|$.
	
	Let the $m^{th}$ edge $(u, v)$ be assigned to subgraph $i$ ($1 \le i \le p$) by algorithm~\ref{alg:greedy}.
	By line $15$ of algorithm~\ref{alg:greedy},
	\begin{equation} 
	\label{equ:inequality_0}
	 Score^m_{(u,v)}(i) - Score^m_{(u,v)}(j) \le 0
	\end{equation}
	
	for any $j \in [1, p], i \ne j$.
	%The superscript $m$ in this proof represents the current value when processing (assigning) the $m^{th}$ edge.
	
	Substitute equation (\ref{equ:eva}) to inequality (\ref{equ:inequality_0}), we obtain 
	\begin{equation} 
	\label{equ:inequality}
	\begin{aligned}
	\alpha \frac{e_{count}^m[i] - e_{count}^m[j]}{|E| / p} \le& \beta \frac{v_{count}^m[j] - v_{count}^m[i]}{|V| / p} \\
	+ &\mathbb{I}(u \notin keep^m[j]) +\mathbb{I}(v \notin keep^m[j]) \\
	- &\mathbb{I}(u \notin keep^m[i]) - \mathbb{I}(v \notin keep^m[i]).
	\end{aligned}
	\end{equation}
	
	Indicator function $\mathbb{I}(State)$ is a boolean function. Therefore, the upper bound of $\mathbb{I}(u \notin keep^m[j]) + \mathbb{I}(v \notin keep^m[j]) - \mathbb{I}(u \notin keep^m[i]) - \mathbb{I}(v \notin keep^m[i])$ is $2$.
	Meanwhile, since $0 \le v_{count}^m[i], v_{count}^m[j] \le |V|$, $|v_{count}^m[i] - v_{count}^m[j]| \le |V|$.
	Applying these inequalities to equation (\ref{equ:inequality}), the following equation 
	\begin{equation} 
	\label{equ:inequality_2}
	\begin{aligned}
	 e_{count}^m[i] - e_{count}^m[j] \le \frac{2|E|}{\alpha p} + \frac{\beta}{\alpha} |E|
	\end{aligned}
	\end{equation}
	holds.
	
	Since $e_{count}^m[i]$ and $e_{count}^m[j]$ are integers, equation (\ref{equ:inequality_2}) can be rewritten as 
	\begin{equation} 
	\label{equ:inequality_3}
	\begin{aligned}
	e_{count}^m[i] - e_{count}^m[j] \le \lfloor \frac{2|E|}{\alpha p}  + \frac{\beta}{\alpha} |E| \rfloor .
	\end{aligned}
	\end{equation}

	\begin{lemma}
		For any $i, j$ satisfy $1 \le i \ne j \le p$, $e_{count}^m[i] - e_{count}^m[j] \le 1 + \lfloor \frac{2|E|}{\alpha p}  + \frac{\beta}{\alpha} |E| \rfloor$ holds for any $m \in [1, |E| + 1]$.
	\end{lemma}

	\begin{proof}
		If there exists any $i$, $j$ such that $e_{count}^m[i] - e_{count}^m[j] \ge 1 + \lfloor \frac{2|E|}{\alpha p}  + \frac{\beta}{\alpha} |E| \rfloor$, equation (\ref{equ:inequality_3}) indicates that the new edge will not be assigned to subgraph $i$.
		Therefore, for any $m \in [1, |E|]$
		\begin{equation} 
		e_{count}^{m+1}[i] - e_{count}^{m+1}[j] \le e_{count}^m[i] - e_{count}^m[j]
		\end{equation}
		when $e_{count}^m[i] - e_{count}^m[j] \ge 1 + \lfloor \frac{2|E|}{\alpha p} + \frac{\beta}{\alpha} |E| \rfloor$.
		
		Besides, for any $i \in [1, p]$, $e_{count}^1[i] = 0$.

		Thus, the lemma can be proved by mathematical induction. For the sake of brevity, we omit the details.
	\end{proof}
	
	Since $e_{count}^{|E| + 1}[i] = |E_i|$ and $\sum_{i = 1}^p |E_i| = |E|$,
	\begin{equation} 
	\label{equ:prove_1}
	\begin{aligned}
	\sum_{j = 1}^p (|E_i| - |E_j|) = & p \times |E_i| - |E|
	\end{aligned}
	\end{equation}
	for any $i$.
	
	By lemma 1,
	\begin{equation} 
	\label{equ:prove_2}
	\begin{aligned}
	\sum_{j = 1}^p	(|E_i| - |E_j|)& = \sum_{j = 1, j \ne i}^p (|E_i| - |E_j|) \\
	& \le (p -1) \times (1 + \lfloor \frac{2|E|}{\alpha p} + \frac{\beta}{\alpha} |E| \rfloor).
	\end{aligned}
	\end{equation}
	
	Substitute equation (\ref{equ:prove_1}) to (\ref{equ:prove_2}),
	\begin{equation} 
	\label{equ:prove_3}
	\begin{aligned}
	\frac{|E_i|}{|E|/p} \le 1 + \frac{p-1}{|E|} (1 + \lfloor \frac{2|E|}{\alpha p} + \frac{\beta}{\alpha} |E| \rfloor)
	\end{aligned}
	\end{equation}
	for any $i \in [1, p]$.
	Thus we have $\frac{\max_{i=1,...,p} |E_{i}|}{|E|/p} \le 1 + \frac{p-1}{|E|} (1 + \lfloor \frac{2|E|}{\alpha p} + \frac{\beta}{\alpha} |E| \rfloor)$.
	
\end{proof}

\begin{theorem}
	Partitioning graph $G(V, E)$ into $p$ partitions by our EBG algorithm, the upper bound of the vertex imbalance factor is $1 + \frac{p-1}{\sum_{j = 1}^p|V_j|} (1 + \lfloor \frac{2|V|}{\beta p}  + \frac{\alpha}{\beta} |V| \rfloor)$.
\end{theorem}
	
The proof of theorem 2 adopts the same method used in the proof of theorem 1 with minor modifications.
For the sake of simplicity, we do not present it in this paper.

\section{}\label{app:cal}
Figure~\ref{fig:part} demonstrates the partition results of EBG.
We will show the detailed calculation steps of edge assignments here.
In this case, we set $\alpha$ and $\beta$ as the default value $1$.

First, we calculate the degree of each vertex and sort edges in ascending order by the sum of their two end-vertices' degrees.
\begin{table}[htb]
	\caption{Edge order calculation}
	%\protect\\	
	%The column ``Sum of degrees'' presents the calculation step of each edge.}
	\label{tab:sum_degree}
	\centering
	\begin{tabular}{@{}ccc@{}}
		Edge & Sorting index & Sum of end-vertices' degrees \\ \midrule
		$(B, C)$ & $1$ & $degree[B] + degree[C] = 2 + 2 = 4$ \\ 
		$(A, E)$ & $2$ & $degree[A] + degree[E] = 5 + 1 = 6$ \\
		$(A, F)$ & $3$ & $degree[A] + degree[F] = 5 + 1 = 6$ \\
		$(A, D)$ & $4$ & $degree[A] + degree[D] = 5 + 1 = 6$ \\
		$(A, B)$ & $5$ & $degree[A] + degree[E] = 5 + 2 = 7$ \\
		$(A, C)$ & $6$ & $degree[A] + degree[E] = 5 + 2 = 7$ \\
		\bottomrule
	\end{tabular}
\end{table}

Table~\ref{tab:sum_degree} shows the order of edges by the sum of end-vertices' degrees.
%For edges with the same sum of end-vertices' degrees, we sort them in arbitrary order.
Next, we calculate the edge assignments by the order in table~\ref{tab:sum_degree}.
The evaluation function $Score_{(u, v)}(i)$ is defined in equation (\ref{equ:eva}).
Detailed calculation steps for EBG are shown in table~\ref{tab:ebg}.

\begin{table}[htb]
	\caption{EBG edge assignments \protect\\
		Table~\ref{tab:ebg} shows calculation step of EBG. The column ``Evaluation function'' is written in format $(\mathbb{I}(u \notin keep[i]) + \mathbb{I}(v \notin keep[i]) ) + \alpha \frac{e_{count}[i]}{|E| / p} + \beta \frac{v_{count}[i]}{|V|/p}$}
	\label{tab:ebg}
	\centering
	\begin{tabular}{@{}ccccc@{}}\toprule
		& & \multicolumn{2}{c}{\emph{Evaluation function}} &  \\
		\cmidrule(lr){3-4} 
		Edge & Index & Subgraph $0$ & Subgraph $1$ & Assignment \\ \midrule
		$(B, C)$ & $1$ & $2 + \frac{0}{3} + \frac{0}{3} = 2$ & $2 + \frac{0}{3} + \frac{0}{3} = 2$ & $1$ \\ 
		$(A, E)$ & $2$ & $2 + \frac{0}{3} + \frac{0}{3} = 2$ & $2 + \frac{1}{3} + \frac{2}{3} = 3$ & $0$ \\
		$(A, F)$ & $3$ & $1 + \frac{1}{3} + \frac{2}{3} = 2$ & $2 + \frac{1}{3} + \frac{2}{3} = 3$ & $0$ \\
		$(A, D)$ & $4$ & $1 + \frac{2}{3} + \frac{3}{3} = \frac{8}{3}$ & $2 + \frac{1}{3} + \frac{2}{3} = 3$ & $0$ \\
		$(A, B)$ & $5$ & $1 + \frac{3}{3} + \frac{4}{3} = \frac{10}{3}$ & $1 + \frac{1}{3} + \frac{2}{3} = 2$ & $1$ \\
		$(A, C)$ & $6$ & $1 + \frac{3}{3} + \frac{4}{3} = \frac{10}{3}$ & $0 + \frac{2}{3} + \frac{3}{3} = \frac{5}{3}$ & $1$ \\
		\bottomrule
	\end{tabular}
\end{table}
